# Supplementary material for: A note on the Burris-Willard conjecture
Source: arXiv:2011.09027 ancillary file (2020-11-18)
Supplement: Supplementary file 1 [file short_description_of_files.pdf]

## Short overview of the ancillary files

The top directory `anc/` contains:

**short\_description\_of\_files.pdf** This file.

**cpp/** A subdirectory containing `c++`-source, input and output files, mainly pertaining to Remark 13 (also Lemmata 4, 6 and 12) and Section 4 (in particular Algorithm 18 and Example 19) in the paper. There are two subdirectories according to the division between Section 3 and Section 4:

**commutation-with-T/** Content related to Section 3.

**commutationTs.cpp** This is `c++`-code containing several functions in connection with the centraliser of Snow's quaternary function  $T$  on the set  $\{0, 1, 2\}$ .

The code is documented in the file `commutationTs.cpp` itself. For many functions in this file standard output needs to be redirected to a file in order to save the results, see also the description of the subsequent output files in the same directory. The main output generating functions are the following:

**findallunaries()** outputs  $\{T\}^{*(1)}$ , the result of which can be found in `Tcent1.txt`.

**findallbinaries()** outputs  $\{T\}^{*(2)}$ , the result of which can be found in `Tcent2.txt`.

**writeallbinariesforz3()** outputs  $\{T\}^{*(2)}$  in a format to be used as part of `func_Tc2c2.z3`.

**findallternaries\_optimised()** outputs  $\{T\}^{*(3)}$  according to the strategy described in Remark 13. After sorting, the result is the long file `Tcent3_sorted.txt`.

**readTcent3(char const\* fname)** reads 1 048 578 ternary operations from the file named `fname` and checks whether all of these commute with the binary operation  $f$  from Lemma 12. Calling `readTcent3("Tcent3_sorted.txt")` proves that  $f \in \{T\}^{*(3)*(2)}$  as claimed in Remark 13.

**Tcent1.txt** This file contains all functions of  $\{T\}^{*(1)}$  for the case  $k = 3$ , to substantiate the content of Lemma 4. This output file is produced by the function `findallunaries()` from `commutationTs.cpp` and redirecting standard output.

**Tcent2.txt** This file contains all functions of  $\{T\}^{*(2)}$  for the case  $k = 3$ , which verifies Lemma 6. This output file is produced by the function `findallbinaries()` from `commutationTs.cpp` and redirecting standard output.

**Tcent3\_sorted.txt** This file contains all 1 048 578 functions of  $\{T\}^{*(3)}$  for  $k = 3$ , as mentioned in Remark 13. This output file is produced by the function `findallternaries_optimised()` from `commutationTs.cpp`, redirecting standard output and then sorting it. It is the input that one needs to use for the function `readTcent3("Tcent3_sorted.txt")` when verifying that the function  $f$  from Lemma 12 satisfies  $f \in \{T\}^{*(3)*(2)}$  as claimed in Remark 13. As  $\{T\}^{*(3)*(2)} \subseteq \{T\}^{*(2)*(2)}$ , this calculation also confirms part of the statement of Lemma 12.

**find-ppdefinitions/** Content related to Section 4.

This directory contains an implementation of (the central part of) Algorithm 18 from the paper (see `ppdefinitions.cpp`), which attempts to compute a primitive positive definition of a relation in a finitely generated relational clone. This implementation may be useful independently of questions relating to the function  $T$  or centraliser clones.

After compilation, the programme expects to read a file named `input.txt` in the same directory, containing the relations generating the relational clone and a generating system of the relation to be represented by a primitive positive formula. The input format is explained in `input_template.txt`. The goal relation (or its generating system) is *not allowed* to have *duplicate coordinates*, that is, if the tuples of the relation are represented as columns of a matrix, this matrix is not allowed to have any two identical rows. This slightly simplifies the implementation and is not a severe restriction in most practical cases: one may project away duplicate coordinates before and may manually modify the formula at the end. After termination (which may take a long time), the programme outputs two files containing the representing formula: `ppoutput.out` and `checkppoutput.z3`. If a proper subrelation is used as a generating system of the goal relation, then the latter file needs to be modified by hand in order to work correctly. Namely,

the definition of the goal relation  $S$  in `checkppoutput.z3` has to be completed by all its tuples, not just those from the generating subrelation that were automatically added by the programme.

**compile.sh** A POSIX compatible shell script compiling the source file `ppdefinitions.cpp` into an executable `getppformula` using `g++` as its compiler.

**input\_2generated.txt** An input file that may be copied onto `input.txt` to be read by `getppformula` to perform the computations described in Example 19 of the paper. The result of this run is contained in the files `ppoutput_2generated.out` and `checkppoutput_2generated.z3` (in the `anc/z3/` directory), which prove the fact  $f \in \{T\}^{**}$  from Lemma 14.

**input\_template.txt** This is the template file that explains how the relations need to be communicated to the programme `getppformula`. The template should never be modified, but is intended to be copied onto `input.txt`, which should then be adapted to any particular use case.

**input.txt** This is the actual input file that is read by the executable obtained from `ppdefinitions.cpp`. In the current submission, it is identical to `input_2generated.txt` relating to Example 19 in the paper, but one may modify it to solve any other problem.

**ppdefinitions.cpp** This is an implementation of Algorithm 18 from the paper in `c++11`, except for the preprocessing step that takes care to transform  $\gamma_0$  into  $\gamma$  without duplicate coordinates and to define the map  $\alpha$  (lines 2–9). The programme reads `input.txt` and outputs `ppoutput.out` and `checkppoutput.z3` containing the desired formula. The file `ppoutput.out` is a simple ascii text while `checkppoutput.z3` is a script that can be used to check the correctness of the computation with the Z3 theorem prover. Do not forget to *manually expand* `checkppoutput.z3` if using a proper generating system for the goal relation that is to be described by a primitive positive formula.

**ppoutput\_2generated.out** This file contains the output of the executable `getppformula` when run on the configuration specified in `input_2generated.txt`, i.e., it contains the result of the computations in Example 19 in the paper: a primitive positive formula with six existentially quantified variables and 6 561 atoms showing that  $f \in \{T\}^{**}$  (cf. Lemma 14).

**z3/** A subdirectory containing **z3**-script files to be fed into the Z3 theorem prover (find the source code at <https://github.com/z3prover/z3> or see <https://rise4fun.com/Z3/> for an interactive version) in order to verify various statements made in the paper. These files are:

**binaryfunccommutingT.z3** A script to verify the truth of Lemma 6 and its proof.

**checkformulaforbinfunc.z3** A script to verify the correctness of the primitive positive formula exhibited in Lemma 14 to describe  $f^\bullet$  from Lemma 12 in terms of  $T^\bullet$ .

**checkppoutput\_2generated.z3** This script is the output of the programme `ppdefinitions.cpp` in `anc/cpp/find-ppdefinitions/` run on the content of `input_2generated.txt` as its input file `input.txt` (the definition of  $\mathbf{S}$  was corrected after the computation). The script may be used to check that the automatically computed primitive positive formula expressing the graph  $f^\bullet$  (see Lemma 12) using 6 561 atoms of  $T^\bullet$  does indeed, what it is supposed to do. Hence, this file substantiates the results claimed in Example 19 of the paper, and it provides a different proof why  $f \in \{T\}^{**}$  (cf. Lemma 14).

**func\_Tc2c2.z3** A script to verify the correctness of Lemma 12, in particular the final part of its proof: i.e., that the binary function  $f$  from Lemma 12 indeed commutes with all 65 functions listed in Lemma 6, and also that it is unique with respect to this property under the assumption of not belonging to the binary part of the clone generated by  $T$ .

**unaryfunccommutingT.z3** A script to verify the truth of Lemma 4 for the case  $k = 3$ .
